# Supplementary material for: Border-SegGCN: Improving Semantic Segmentation by Refining the Border Outline using Graph Convolutional Network
Source: arXiv:2109.05353 source file (2021-09-11)
Supplement: Supplementary file 1 [file supplement.pdf]

# Border-SegGCN: Improving Semantic Segmentation by Refining the Border Outline using Graph Convolutional Network: Supplementary Material

Naina Dhingra, George Chogovadze, Andreas Kunz

ETH Zurich

## 1 Results

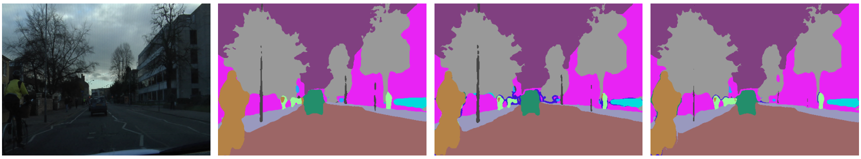

(a) (b) (c) (d)

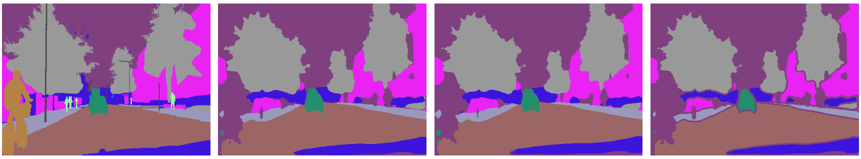

(e) (f) (g) (h)

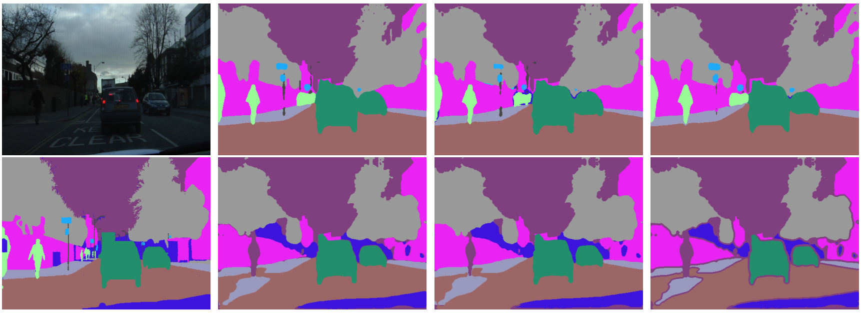

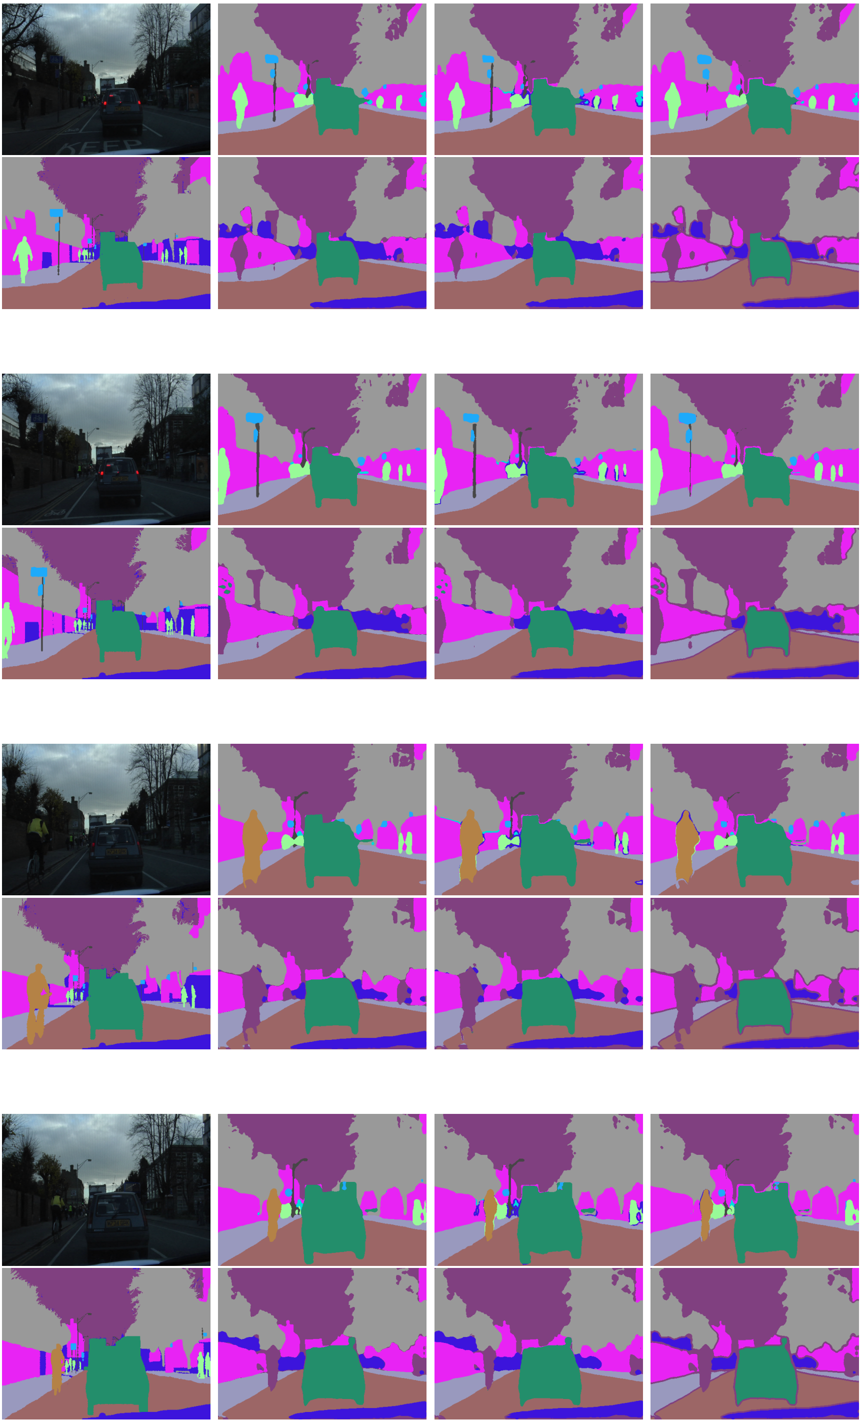

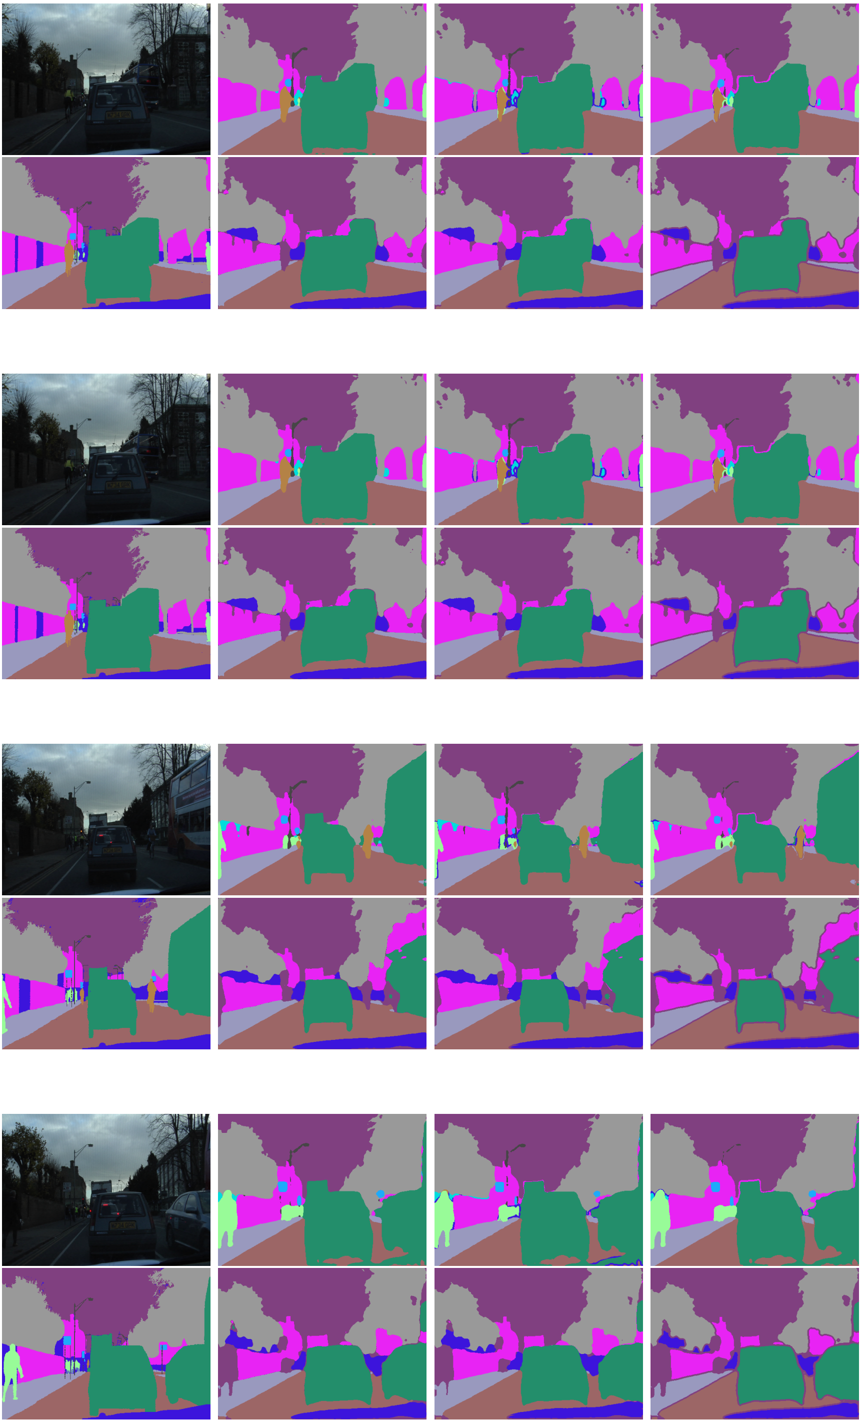

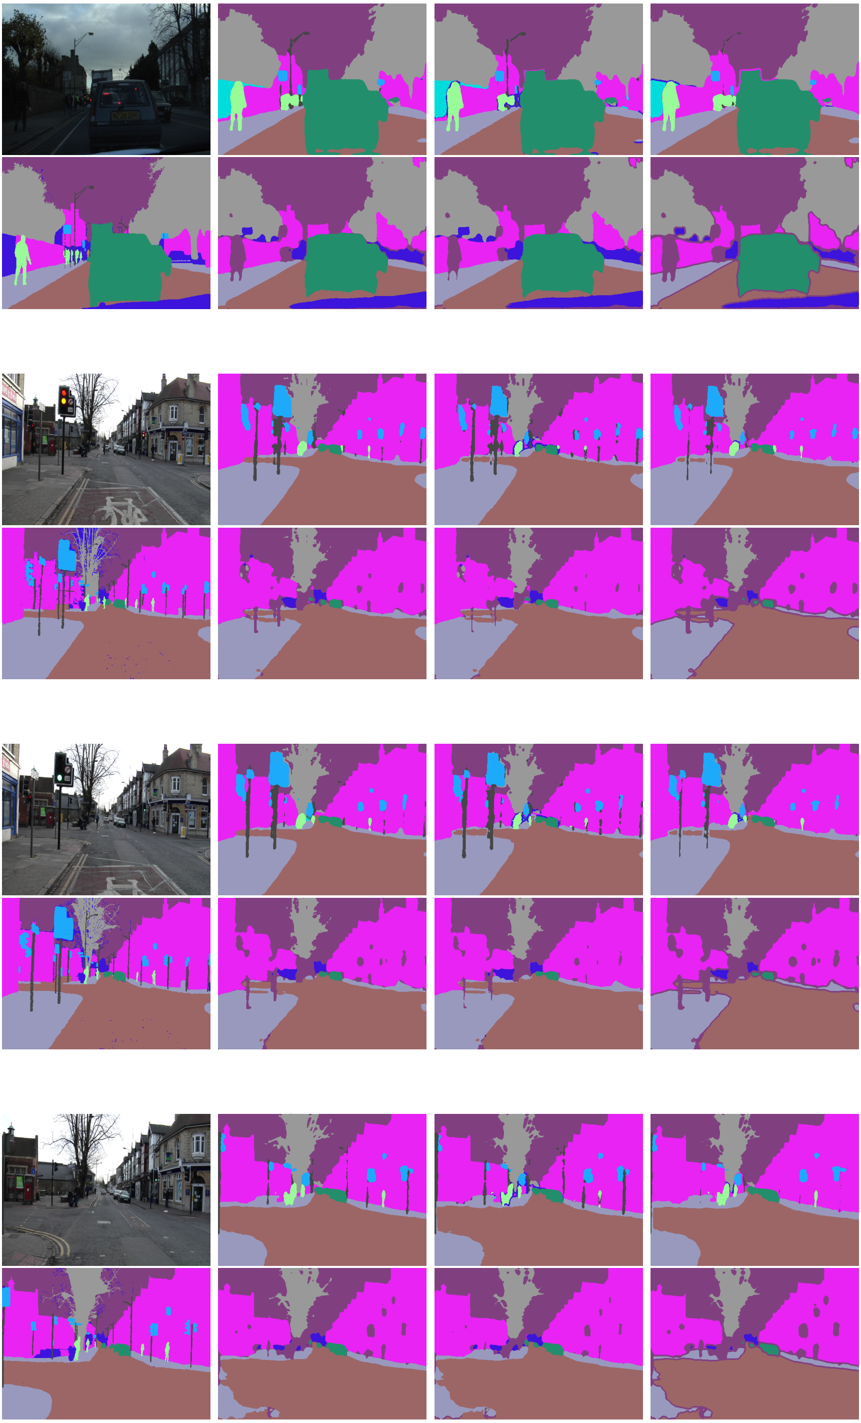

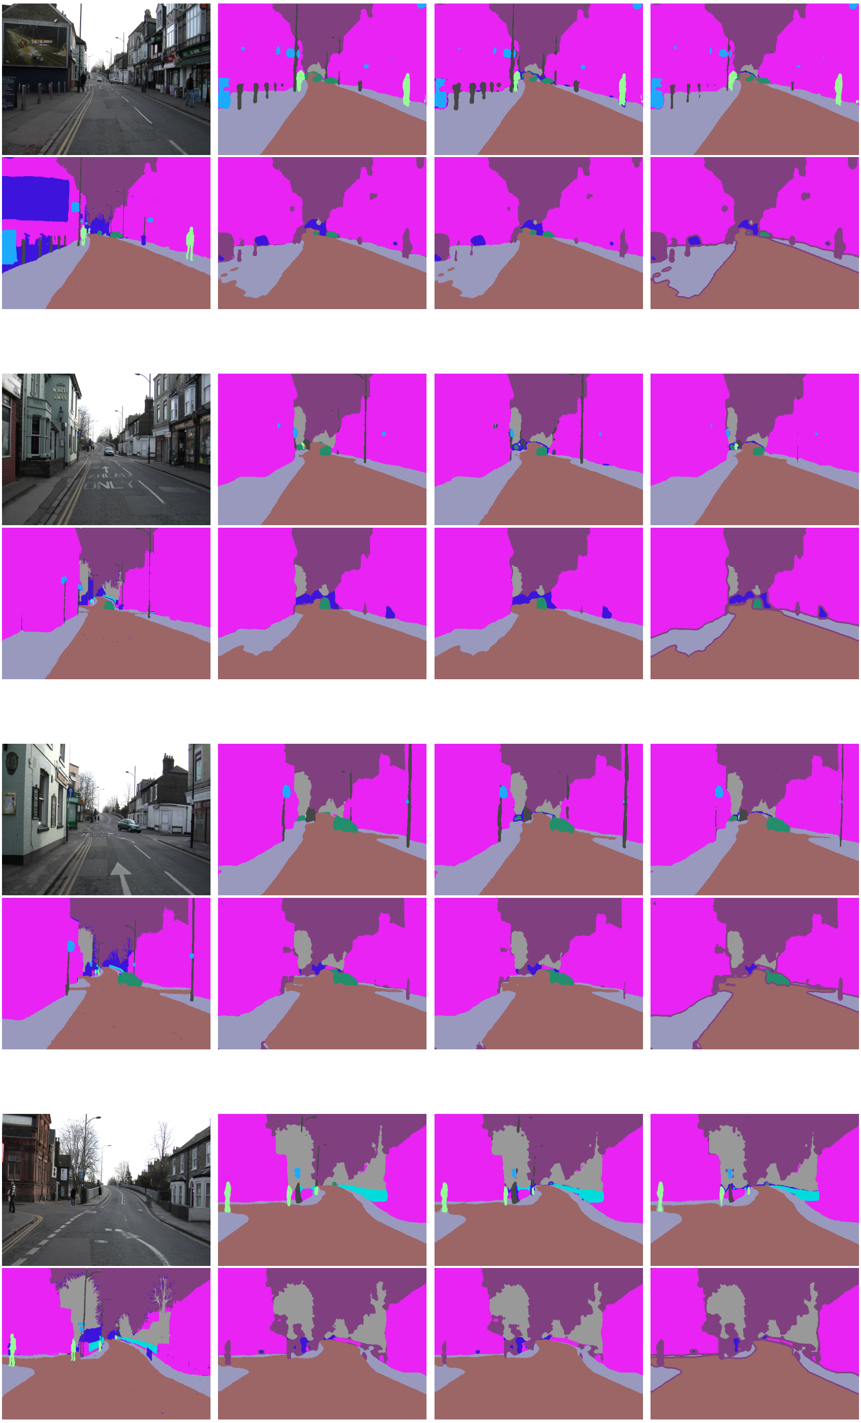

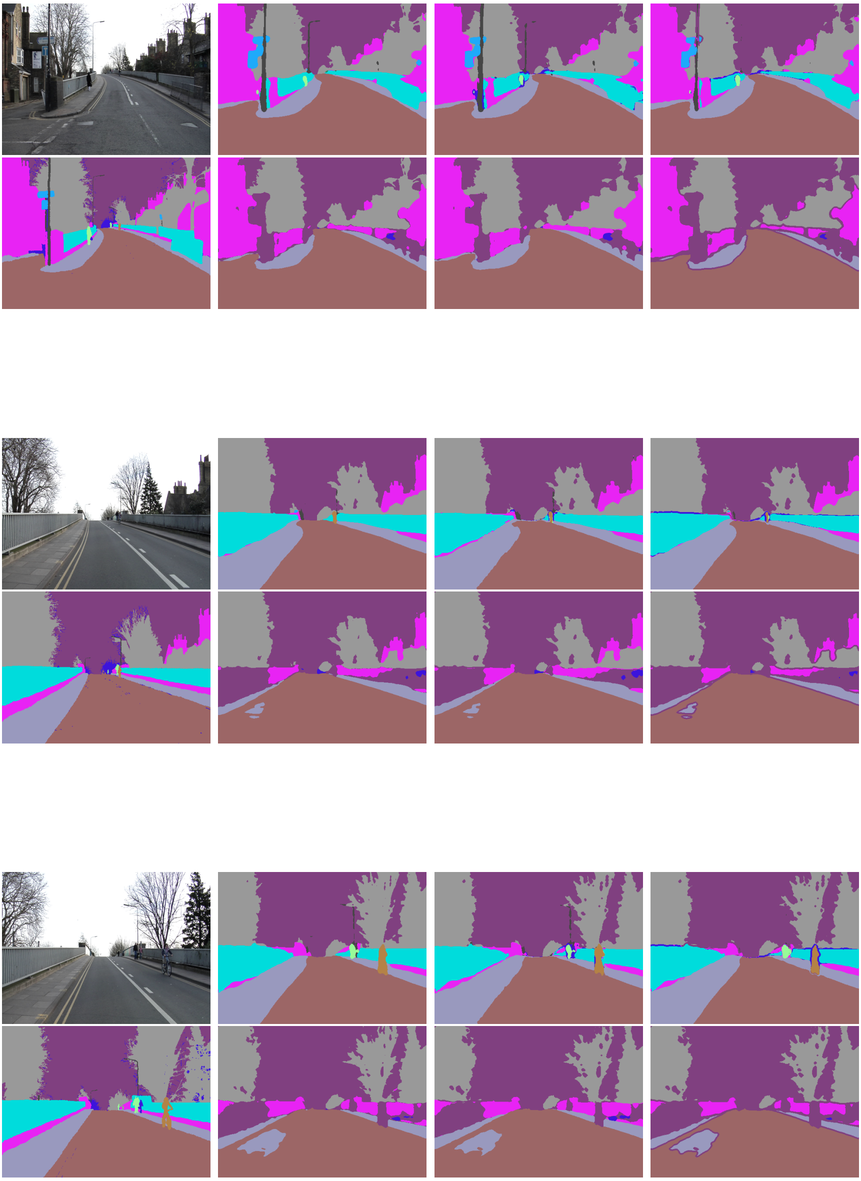

**Fig. 1.** Results of our Border-SegGCN on various frames from CamVid dataset. (a) Original. (b) DeepLabV3+ baseline. (c) Best Border-SegGCN with DeepLabV3+. (d) Poor Border-SegGCN with DeepLabV3+. (e) Ground truth. (f) Unet baseline. (g) Best Border-SegGCN with Unet. (h) Poor Border-SegGCN with Unet. All the following examples follow the same structure as the first example.

# 2 Image to graph

In this section, we will describe two approaches to generate a graph from an image which we have implemented and evaluated with experiments.

## 2.1 Nodes

Each pixel in an image can be interpreted as a node with three feature channels corresponding to the red, green and blue channels.

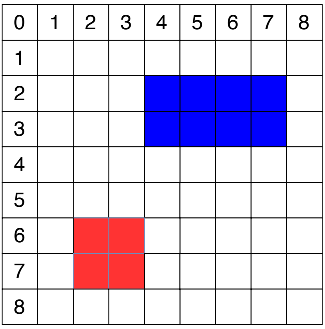


**Fig. 2.** Division of an image into a pixel grid. Each pixel represents a node.

## 2.2 Labels

The node label would be the class that the corresponding pixel belongs to. Identifying the label of each node is identical to semantically segmenting the image. Figure 3 illustrates how the labels would be associated if we take as an example. Figure 2. Each box in the grid has now a label relating it either to a cube, background or rectangle. Notice here we chose to illustrate this with the ground truth as such there is no mismatch between the label and the actual image.

| 0 | 1 | 2 | 3 | 4 | 5 | 6 | 7 | 8 |
|---|---|---|---|---|---|---|---|---|
| 1 | B | B | B | B | B | B | B | B |
| 2 | B | B | B | R | R | R | R | B |
| 3 | B | B | B | R | R | R | R | B |
| 4 | B | B | B | B | B | B | B | B |
| 5 | B | B | B | B | B | B | B | B |
| 6 | B | C | C | B | B | B | B | B |
| 7 | B | C | C | B | B | B | B | B |
| 8 | B | B | B | B | B | B | B | B |

**Fig. 3.** Ground truth associated with each node as the "label" attribute. "R" represent rectangle. "C" represents cube. "B" represents background.

## 2.3 Connections

The interconnection of nodes is required to connect the nodes to have a structure. One way is to connect each node to its closest spatial neighbours to simulate the characteristics of an image. For example, each node would have connection going to its 4, 8, 24, ... closest spatial neighbours as shown in Figure 4. This choice would allow the retention of information concerning the spatial dependency between the pixels. Another way is to consider the similarity that two pixels have

| 0 | 1 | 2 | 3 | 4 | 5 | 6 | 7 | 8 |
|---|---|---|---|---|---|---|---|---|
| 1 | | | | | | | | |
| 2 | | 24C | 24C | 24C | 24C | 24C | | |
| 3 | | 24C | 8C | 4C | 8C | 24C | | |
| 4 | | 24C | 4C | S | 4C | 24C | | |
| 5 | | 24C | 8C | 4C | 8C | 24C | | |
| 6 | | 24C | 24C | 24C | 24C | 24C | | |
| 7 | | | | | | | | |
| 8 | | | | | | | | |

**Fig. 4.** Closest neighbours of a particular node. In this case "S" is the central node. Each value in the case represents to which group of closest neighbours it belongs to e.g. "8C": 8 closest neighbours.

| 0 | 1 | 2 | 3 | 4 | 5 | 6 | 7 | 8 |
|---|---|---|---|---|---|---|---|---|
| 1 | | | | | | | | |
| 2 | | $\sqrt{8}$ | $\sqrt{5}$ | 2 | $\sqrt{5}$ | $\sqrt{8}$ | | |
| 3 | | $\sqrt{5}$ | $\sqrt{2}$ | 1 | $\sqrt{2}$ | $\sqrt{5}$ | | |
| 4 | | 2 | 1 | 0 | 1 | 2 | | |
| 5 | | $\sqrt{5}$ | $\sqrt{2}$ | 1 | $\sqrt{2}$ | $\sqrt{5}$ | | |
| 6 | | $\sqrt{8}$ | $\sqrt{5}$ | 2 | $\sqrt{5}$ | $\sqrt{8}$ | | |
| 7 | | | | | | | | |
| 8 | | | | | | | | |

| 0 | 1 | 2 | 3 | 4 | 5 | 6 | 7 | 8 |
|---|---|---|---|---|---|---|---|---|
| 1 | | | | | | | | |
| 2 | | | | 0.5 | | | | |
| 3 | | | | 0.5 | | | | |
| 4 | | 0.25 | 0.5 | S | 1 | 0.5 | | |
| 5 | | | | 1 | | | | |
| 6 | | | | 0.25 | | | | |
| 7 | | | | | | | | |
| 8 | | | | | | | | |

**Fig. 5.** Left: Euclidean weights for 25 closest neighbours of pixel (4, 4). Right: Weights taking into account euclidean distance and RGB value differences.

with each other in combination with the distance between them, similar to [2]. So, we used a mapping that is dependant on the Euclidean distance and pixel channel similarities to cast the result between 0 and 1.

## 2.4 Features

The feature matrix with the adjacency matrix is used by GCN to determine if a certain pixel belongs to one class or another. Thus, it is crucial to select the right features for each node. Feature set includes intensity of RGB channels, base algorithm predicted output as shown in Figure 6 to improve the pre-segmented image, and intermediate feature values from the base network such as Unet as shown in Figure7.

| 0 | 1 | 2 | 3 | 4 | 5 | 6 | 7 | 8 |
|---|---|---|---|---|---|---|---|---|
| 1 | B | B | B | B | B | B | B | B |
| 2 | B | B | R | R | R | R | R | B |
| 3 | B | B | R | R | C | R | R | B |
| 4 | B | B | B | R | R | B | B | B |
| 5 | B | B | B | B | B | B | B | B |
| 6 | B | C | C | B | B | B | B | B |
| 7 | B | C | B | B | B | B | B | B |
| 8 | B | B | B | B | B | B | B | B |

**Fig. 6.** Output from a base algorithm that Border-SegGCN would build on. Notice that the labels do not always match the truth.

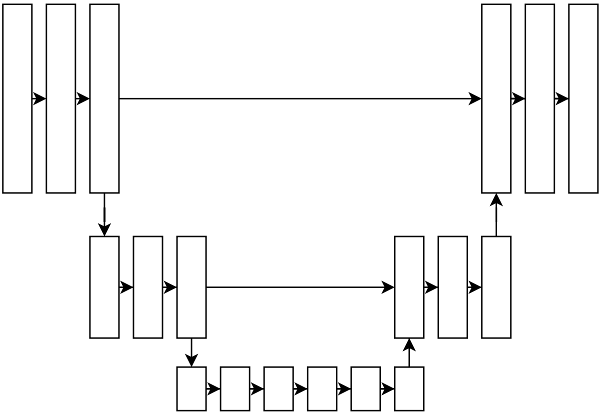

**Fig. 7.** Simple overview of the Unet architecture. The output of each intermediary layer can be used as a feature set.

## 3 Graph size

In 100px x 100px image will have 100'00 pixels. This can result in very large graphs and thus large dense adjacency matrices. Furthermore, if the intermediate layers are used as features sets, the feature matrices can also become quite large. Thus, it is important to consider selective pixel criteria for the graph creation. Semantic segmentation is quite problematic on the boundaries that lay between

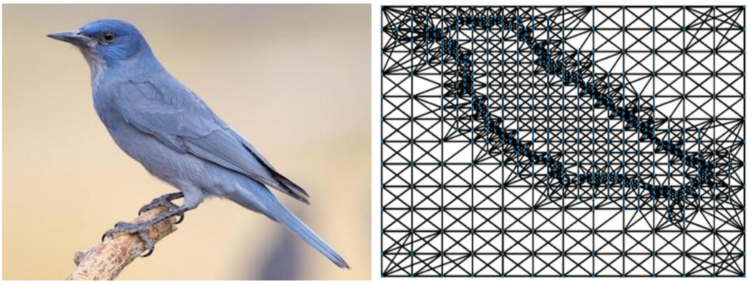

**Fig. 8.** Left: Original image [1]. Right: Graph obtained by introducing a bias on the border. Each node is connected to its 8 closest neighbours.

objects of different classes. So, we select pixels that are around the boundary to perform processing and classification on them. Figure 8 shows a concrete example of variable meshing that we studied for an image. This however introduces a problem with regards to topology. The GCN requires that the size of the adjacency matrix stay the same from graph to graph. This implies that the number of nodes need to stay constant in each frame.

A solution to variable sized graphs as shown in Figure 9 is the concatenation of these graphs into a "supergraph" as described by [3]. Although, it is possible to perform node classification with variable size graphs using supergraph, it is no longer possible to separate different kinds of frames as shown in Figure 10 . Thus rendering training, validation and testing inseparable. This would prohibit the segmentation of new frames and all data needs to be provided before hand. As the number of frames are stacked, although sparse, the super graph still becomes quite large leading to memory issues. The solution to this problem is used and described in our paper.

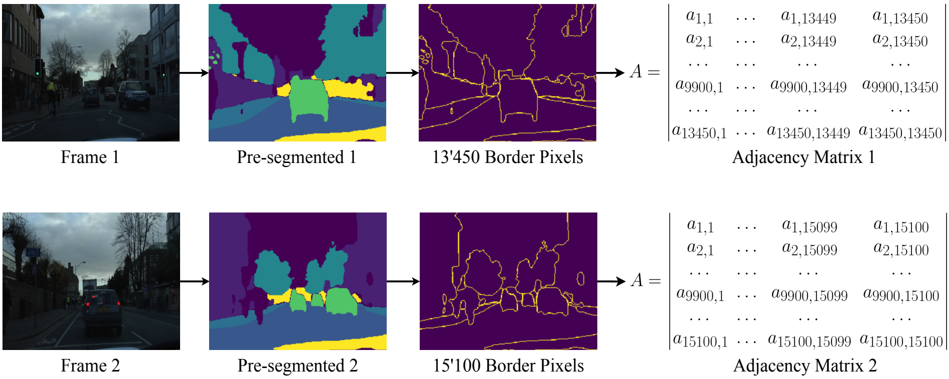


**Fig. 9.** Topological mismatch between the adjacency matrices of 2 frames in the event of only selecting border pixels.

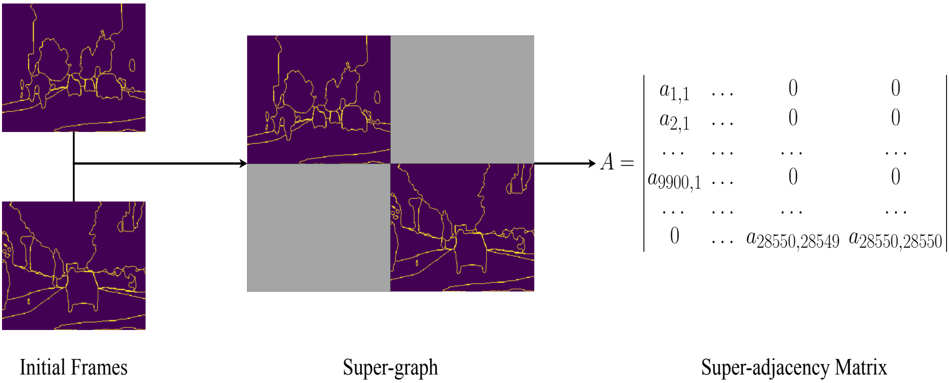


**Fig. 10.** Pipeline for concatenating images with the goal to solve the topological constraint on the adjacency matrix.

## References

1. Pinyon jay bird, "https://independent.co.uk"
2. Boykov, Y., Funka-Lea, G.: Graph cuts and efficient nd image segmentation. International Journal of Computer Vision - IJCV **70**, 109–131 (11 2006). https://doi.org/10.1007/s11263-006-7934-5
3. Kipf, T.N., Welling, M.: Semi-supervised classification with graph convolutional networks. CoRR **abs/1609.02907** (2016), http://arxiv.org/abs/1609.02907
